# Supplementary material for: Can Agents Learn by Analogy? An Inferable Model for PAC Reinforcement Learning
Source: arXiv:1912.10329 source file (2020-02-24)
Supplement: Supplementary file 1 [file whitening.tex]

%!TEX root = ../0_neurips19_tensor_rl_main.tex

\subsection{Symmetrization}
\label{apd:symm}

Suppose we have an asymmetric third order tensor $\mytensor{M} \in \mathbb{R}^{I \times J \times K}$, which has the CP form $\mytensor{M} = \sum_{r=1}^R \lambda_r \boldsymbol{a}_r \otimes \boldsymbol{b}_r \otimes \boldsymbol{c}_r$. We can convert $\mytensor{M}$ into a symmetric tensor $\mytensor{F} \in \mathbb{R}^{K \times K \times K}$ with CP form $\mytensor{F} =  \sum_{r=1}^R \omega_r \boldsymbol{c}_r \otimes \boldsymbol{c}_r \otimes \boldsymbol{c}_r$ with the following steps.

\textbf{Step 1: linear combination of slices}

Choose a vector $\myvector{v}_c \in \mathbb{R}^K$, and get

\begin{align}
	\mymatrix{M}_{ab}^{v_c} := \mytensor{M}(I,I,\myvector{v_c}) = \sum_{r=1}^R \lambda_r <\myvector{v_c}, \myvector{c}_r> \myvector{a}_r \otimes \myvector{b}_r = \mymatrix{U_a} \mymatrix{\Sigma_{ab}^{v_c}} \mymatrix{U_b}\tran \\
	\mymatrix{M}_{ba}^{v_c} := \mytensor{M}(I,I,\myvector{v_c})\tran = \sum_{r=1}^R \lambda_r <\myvector{v_c}, \myvector{c}_r>  \myvector{b}_r \otimes \myvector{a}_r= \mymatrix{U_b} \mymatrix{\Sigma_{ba}^{v_c}} \mymatrix{U_a}\tran
\end{align}

This is equivalent with constructing a matrix by linearly combining the frontal slices with the weight vector $\myvector{v}$. Similarly, we can obtain $\mymatrix{M}_{ac}^{v_b} := \mytensor{M}(I,\myvector{v_b},I)$, $\mymatrix{M}_{bc}^{v_a} := \mytensor{M}(\myvector{v_a},I, I)$ and so on.

\textbf{Step 2: projection}

Find matrices $\mymatrix{A} \in \mathbb{R}^{R \times I}$ and $\mymatrix{B} \in \mathbb{R}^{R \times J}$ such that $\mymatrix{A} \mymatrix{M}_{ab}^{v_c} \mymatrix{B}\tran$ is invertible. Note that $\mymatrix{A} \mymatrix{M}_{ab}^{v_c} \mymatrix{B}\tran = \mymatrix{A} \mymatrix{U_a} \mymatrix{\Sigma_{ab}^{v_c}} \mymatrix{U_b}\tran \mymatrix{B}\tran = (\mymatrix{\Sigma_{ab}^{v_c}})^{\frac{1}{2}} \mymatrix{A} \mymatrix{U_a} ((\mymatrix{\Sigma_{ab}^{v_c}})^{\frac{1}{2}} \mymatrix{B}\mymatrix{U_b})\tran$, so $\mymatrix{A} \mymatrix{U_a}$ and $\mymatrix{B}\mymatrix{U_b}$ are also invertible.

Then set:
\begin{align}
	\tilde{\mymatrix{M}}_{ab} &:= \mymatrix{A} \mymatrix{M}_{ab}^{v_c} \mymatrix{B}\tran \\
	\tilde{\mymatrix{M}}_{ba} &:= \mymatrix{B} \mymatrix{M}_{ba}^{v_c} \mymatrix{A}\tran \\
	\tilde{\mymatrix{M}}_{cb} &:= \mymatrix{M}_{cb}^{v_a} \mymatrix{B}\tran \\
	\tilde{\mymatrix{M}}_{ca} &:= \mymatrix{M}_{ca}^{v_b} \mymatrix{A}
\end{align}

\textbf{Step 3: symmetrization}

Convert the original tensor to a symmetric one by the operation:

\begin{align*}
	\mytensor{F} &= \mytensor{M} \bigg( \big(\tilde{\mymatrix{M}}_{cb}(\tilde{\mymatrix{M}}_{ab})^{-1} \mymatrix{A} \big)\tran, \big( \tilde{\mymatrix{M}}_{ca}(\tilde{\mymatrix{M}}_{ba})^{-1} \mymatrix{B} \big)\tran, I \bigg) \\
	&= \sum_{r=1}^R \mymatrix{U_c} \mymatrix{\Sigma_{cb}^{v_a}} \mymatrix{U_b}\tran \mymatrix{B}\tran 
		(\mymatrix{A} \mymatrix{U_a} \mymatrix{\Sigma_{ab}^{v_c}} \mymatrix{U_b}\tran \mymatrix{B}\tran)^{-1} \mymatrix{A} \myvector{a}_r \otimes
		\mymatrix{U_c} \mymatrix{\Sigma_{ca}^{v_b}} \mymatrix{U_a}\tran \mymatrix{A}\tran 
		(\mymatrix{B} \mymatrix{U_b} \mymatrix{\Sigma_{ba}^{v_c}} \mymatrix{U_a}\tran \mymatrix{A}\tran)^{-1} \mymatrix{B} \myvector{b}_r \otimes \myvector{c} \\
	&= \sum_{r=1}^R \mymatrix{\Sigma_{cb}^{v_a}} \mymatrix{\Sigma_{ab}^{v_c}} \mymatrix{\Sigma_{ca}^{v_b}} \mymatrix{\Sigma_{	ba}^{v_c}}
		\mymatrix{U_c} (\mymatrix{B} \mymatrix{U_b})\tran
		\big( (\mymatrix{B} \mymatrix{U_b})\tran \big)^{-1} (\mymatrix{A} \mymatrix{U_a})^{-1} \mymatrix{A} \myvector{a}_r \otimes
		\mymatrix{U_c} (\mymatrix{A} \mymatrix{U_a})\tran \big( (\mymatrix{A} \mymatrix{U_a})\tran \big)^{-1} (\mymatrix{B} \mymatrix{U_b})^{-1} \mymatrix{B} \myvector{b}_r \otimes \myvector{c}_r \\
	&= \sum_{r=1}^R \omega_r \myvector{c}_r \otimes \myvector{c}_r \otimes \myvector{c}_r
\end{align*}

where $\{\omega_r\}_{r=1}^R$ are just scalars depending on $\{\lambda_r\}_{r=1}^R$ and the choices of $\myvector{v}$s.

\subsection{Whitening}
\label{apd:whiten}
