# Supplementary material for: Can Agents Learn by Analogy? An Inferable Model for PAC Reinforcement Learning
Source: arXiv:1912.10329 source file (2020-02-24)
Supplement: Supplementary file 3 [file supp_macros.tex]

\newcommand*{\mytensor}[1]{\bm{\mathcal{#1}}}
\newcommand*{\mymatrix}[1]{\bm{#1}}
\newcommand*{\myvector}[1]{\bm{#1}}
\newcommand*{\noise}[1]{\widehat{#1}}
\newcommand*{\mm}{\mymatrix}
\newcommand*{\mv}{\myvector}
\newcommand{\mt}{\mytensor}
\newcommand*{\mmCols}[2]{\mm{#1}_{[#2]}}

% names
\newcommand{\ourmod}{{GIM}\xspace}
\newcommand{\ourmodfull}{{Greedy Inference Model}\xspace}
\newcommand{\dmname}{{dynamic matrix}\xspace}
\newcommand{\dmnames}{{dynamic matrices}\xspace}
\newcommand{\avgrew}{{AvgReward}\xspace}
\newcommand{\pavgrew}{{PostAvgReward}\xspace}
\newcommand{\numepi}{{TotalEps}\xspace}
\newcommand{\walkname}{{$\beta$-curious walking}\xspace}

% about dynamic matrices
\newcommand{\states}{\mathcal{S}}
\newcommand{\actions}{\mathcal{A}}
\newcommand{\dmat}{\mymatrix{M}}
\newcommand{\dmats}{M}
\newcommand{\admat}{\mymatrix{\hat{M}}}
\newcommand{\rdmat}{\mymatrix{\widetilde{M}}}
\newcommand{\rdmats}{\widetilde{M}}
\newcommand{\dmatset}{\{\mymatrix{M}^k\}_{k=1}^{S+1}}
\newcommand{\admatset}{\{\mymatrix{\hat{M}}^k\}_{k=1}^{S+1}}
\newcommand{\rdmatset}{\{\mymatrix{\widetilde{M}}^k\}_{k=1}^{S+1}}
\newcommand{\krange}{1,2,\cdots,S+1}


% about mask
\newcommand{\mask}{\mymatrix{P}^\mathcal{K}}
\newcommand{\masks}{P^\mathcal{K}}
\newcommand{\kset}{\mathcal{K}}
\newcommand{\nkset}{\bar{\mathcal{K}}}

% about noise
\newcommand{\noiset}{\mytensor{Z}}
\newcommand{\noisem}{\mymatrix{Z}}
\newcommand{\noises}{Z}

\newcommand{\fraction}{\rho}

\newcommand{\minsa}{M_{in}}
\newcommand{\maxsa}{M_{ax}}

\DeclareMathOperator*{\minimize}{\text{minimize}}

\DeclareMathOperator*{\argmax}{arg\,max}
\DeclareMathOperator*{\argmin}{arg\,min}

% author comments

\iffalse
\newcommand{\fhcomment}{\textcolor[rgb]{1,0,0}{F: }\textcolor[rgb]{1,0,0}}


\newcommand{\grcomment}{}
\newcommand{\jccomment}{}
\newcommand{\fhcomment}{}
\newcommand{\yycomment}{}


% math commands
\newcommand{\F}{\mathcal{F}}
\newcommand{\Z}{\mathbb{Z}}
\newcommand{\N}{\mathbb{N}}
\newcommand{\R}{\mathbb{R}}
\newcommand{\dd}{\mathrm{d}}
\newcommand{\E}{\mathbb{E}}
\newcommand{\Var}{\text{Var}}

\newcommand{\ff}{{\frac{\sqrt{\epsilon}}{2}}}
\newcommand\inner[1]{\langle #1 \rangle}
\newcommand\supp{\operatorname{supp}}

\newcommand{\fracpartial}[2]{\frac{\partial #1}{\partial  #2}}

\newcommand{\name}{{strict saddle}}
\newcommand{\bigname}{{Strict saddle}}


\newcommand{\Hess}{\nabla^2}
\DeclareMathOperator{\Tr}{Tr}
\newcommand{\tlO}{\tilde{O}}
\newcommand{\tlOmega}{\tilde{\Omega}}
\newcommand{\nameCQ}{ $\alpha_c$-RLICQ }
\newcommand{\BigC}{\mathfrak{S}}

\setmainfont{Corbel}  % This was the font used in the powerpoint template


\setlength{\parskip}{0.3em}

\def\Pbb{{\mathbb P}}
\DeclareMathOperator{\Cum}{C_3}
\def\Ebb{{\mathbb E}}
\DeclareMathOperator{\flatten}{unfold}
\def\tha{{\mbox{\tiny th}}}
\newcommand{\CToep}{{\mathcal{F}}}





\DeclareMathOperator*{\argmax}{argmax}




\fi

\newcommand{\ft}{\frametitle}
\newcommand{\bef}{\begin{frame}}
\newcommand{\eef}{\end{frame}} %strange doesnt work
\newcommand{\beb}{\begin{block}}
\newcommand{\eeb}{\end{block}}
\newcommand{\becs}{\begin{columns}}
\newcommand{\eecs}{\end{columns}}
\newcommand{\bec}{\begin{column}}
\newcommand{\eec}{\end{column}}
\newcommand{\bi}{\begin{itemize}}
\newcommand{\ei}{\end{itemize}}

%presentation specs
\def\tcr{\textcolor{red}}
\def\tcb{\textcolor{blue}}
\def\tcg{\textcolor{green}}
\def\tcw{\textcolor{white}}
\def\tcm{\textcolor{magenta}}
\def\tccyan{\textcolor{cyan}}
\def\tcv{\textcolor{violet}}
\definecolor{dkr}{rgb}{0.6,0.2,0.2}
\definecolor{dkg}{rgb}{0,0.5,0}
\definecolor{dkb}{rgb}{0.0,0.1,0.7}

\def\tcdkb{\textcolor{dkb}}
\def\tcdkg{\textcolor{dkg}}
\def\tcdkr{\textcolor{dkr}}
\def\tcblack{\textcolor{black}}
