# Supplementary material for: Can Agents Learn by Analogy? An Inferable Model for PAC Reinforcement Learning
Source: arXiv:1912.10329 source file (2020-02-24)
Supplement: Supplementary file 4 [file supp_packages.tex]

\usepackage{amsmath}
\usepackage{amsfonts}
\usepackage{amssymb}
\usepackage{mathtools}
\usepackage{xspace}
\usepackage{graphicx}
\usepackage{algorithm}
\usepackage{algorithmicx,algpseudocode}
\usepackage{multirow}
%\usepackage{tikz}
%\usetikzlibrary{bayesnet}
%\usepackage{fontspec}
 \usepackage{color}
 \usepackage{psfrag}
 \usepackage{natbib}
 \usepackage{epstopdf}
 \usepackage{subfig}
 \usepackage{hyperref}
\usepackage{siunitx}
\usepackage[labelformat=empty]{caption}  % Disable figure numbering and labels

\usepackage{tikz}
\usetikzlibrary{fit}
\usetikzlibrary{calc,shapes}
\usetikzlibrary{decorations.pathmorphing} % noisy shapes
\usetikzlibrary{fit}					% fitting shapes to coordinates
\usetikzlibrary{backgrounds}	% drawing the background after the foreground
%pgfplots
\usepackage[utf8]{inputenc}
% \usepackage{fontspec}  % optional
\usepackage{pgfplots}
\pgfplotsset{compat=newest}
\usepgfplotslibrary{groupplots}
\usepgfplotslibrary{dateplot}

\usepackage{tcolorbox}
\usepackage{pgfpages}
