# Supplementary material for: Can Agents Learn by Analogy? An Inferable Model for PAC Reinforcement Learning
Source: arXiv:1912.10329 source file (2020-02-24)
Supplement: Supplementary file 5 [file supp_macros.tex]

\definecolor{mygray}{gray}{0.6}
\newcommand{\mycite}[1]{\textcolor{mygray}{\scriptsize{#1}}}

%\newcommand{\myvector}[1]{\ensuremath{\bm{#1}}}
%\newcommand{\mymatrix}[1]{\ensuremath{\bm{#1}}}
%\newcommand{\mytensor}[1]{\bm{\mathcal{#1}}}
%\newcommand{\tensor}[1]{\bm{\mathcal{#1}}}
\newcommand\Dir{\operatorname{Dir}}
\def\tl{\tilde}

\renewcommand\t{{\scriptscriptstyle\top}}

\newcommand\iideq{\stackrel{\mathclap{\normalfont\mbox{\scriptsize{iid}}}}{=}}
\newcommand\iidsim{\stackrel{\mathclap{\normalfont\mbox{\scriptsize{iid}}}}{\sim}}
\newcommand\aseq{\stackrel{\mathclap{\normalfont\mbox{\scriptsize{a.s.}}}}{=}}
\newcommand\whpeq{\stackrel{\mathclap{\normalfont\mbox{\scriptsize{w.h.p.}}}}{\ =\ }}



%\newcommand{\vectorSub}[2]{\ensuremath{\bm{#1}}_{#2}}	
%\newcommand{\vectorSup}[2]{\ensuremath{\bm{#1}}^{(#2)}}
%\newcommand{\vectorInd}[3]{\ensuremath{\bm{#1}}_{#2}^{(#3)}}
%\newcommand{\matrixSub}[2]{\ensuremath{\bm{#1}}_{#2}}	
%\newcommand{\matrixSup}[2]{\ensuremath{\bm{#1}}^{(#2)}}
%\newcommand{\matrixInd}[3]{\ensuremath{\bm{#1}}_{#2}^{(#3)}}
%\newcommand{\tensorSub}[2]{\ensuremath{\bm{\mathcal{#1}}}_{#2}}	
%\newcommand{\tensorSup}[2]{\ensuremath{\bm{\mathcal{#1}}}^{(#2)}}
%\newcommand{\tensorInd}[3]{\ensuremath{\bm{\mathcal{#1}}}_{#2}^{(#3)}}

%\newcommand{\swapaxes}{\mathsf{swapaxes}}
%\newcommand{\flipaxis}{\mathsf{flipaxis}}

%\newcommand\cpeq{\mathrel{\stackrel{\makebox[0pt]{\mbox{\normalfont\tiny cp}}}{=}}}
%\newcommand\tkeq{\mathrel{\stackrel{\makebox[0pt]{\mbox{\normalfont\tiny tk}}}{=}}}
%\newcommand\tteq{\mathrel{\stackrel{\makebox[0pt]{\mbox{\normalfont\tiny tt}}}{=}}}


\newcommand\asymptoticeq{\stackrel{\mathclap{\normalfont\mbox{\scriptsize{\ensuremath{n\!\!\rightarrow\!\!\infty}}}}}{\quad =\quad }}

\newcommand{\mle}{\ensuremath{{\mathsf{mle}}}}
\DeclareMathOperator{\Triples}{T}
\newcommand\inner[1]{\ensuremath{\langle #1 \rangle}}
 \def\hC{\widehat{C}}
\def\hE{\widehat{E}}
% \def\hF{\widehat{F}}
 \def\hG{\widehat{G}}
  \def\hG{\widehat{J}}
 \def\hk{\widehat{k}}
\def\hl{\widehat{l}}
 \def\hSigma{{\widehat{\Sigma}}}
\DeclareMathOperator{\poly}{poly}

 \def\0{{\bf 0}}

\def\leqst{{\overset{st}{\leq}}}
\def\geqst{{\overset{st}{\geq}}}
\def\geqrh{{\overset{rh}{\geq}}}
\def\geqlr{{\overset{lr}{\geq}}}
\def\eqlr{{\overset{lr}{=}}}
\DeclarePairedDelimiter\norm{\lVert}{\rVert}
\DeclareMathOperator{\atanh}{atanh}
\def\tilomega{{\widetilde{\omega}}}
\def\edoc{\end{document}}

\DeclareMathOperator{\rank}{Rank}
  \DeclareMathOperator{\tw}{tw}
\def\Tsawi{{T_{\mathrm{saw}}(i;G)}}
\DeclareMathOperator{\Deg}{Deg}
\DeclareMathOperator{\aug}{Aug}
\DeclareMathOperator{\watts}{Watts}
\DeclareMathOperator{\girth}{Girth}
\DeclareMathOperator{\PL}{PL}
\DeclareMathOperator{\LP}{LP}
\DeclareMathOperator{\ER}{ER}
\DeclareMathOperator{\reg}{Reg}
%mbox - function definitions
\def\tha{\mbox{\tiny th}}
\DeclareMathOperator{\Det}{Det}
\newcommand{\Var}{\mbox{Var}}
\newcommand{\Cov}{\mbox{Cov}}
\newcommand{\Poiss}{\mbox{${\mbox{Poiss}}$}}
\newcommand{\Diag}{\mbox{${\mbox{Diag}}$}}
\newcommand{\Diam}{\mbox{${\mbox{Diam}}$}}
\def\erf{\mbox{erf}}
\def\erfc{\mbox{erfc}}
\def\qfunc{\mbox{Q}}
\def\myexp{\mbox{e}}
\def\snr{\mbox{\tiny SNR}}
\def\signum{\mbox{sgn}}
\def\Card{\mbox{\small N}}
\def\plim{\mbox{p\,}\lim}
\def\convd{\overset{d}\rightarrow}
\def\convp{\overset{p}\rightarrow}
\newcommand\indep{\protect\mathpalette{\protect\independenT}{\perp}}
\def\independenT#1#2{\mathrel{\rlap{$#1#2$}\mkern2mu{#1#2}}}

%%%%%%%%%%%%%%%%%%%%%%%%%%%%%%%%%%%%%%%%%%%%%%%%%%%%%%%%%%%%%%%

%text abbreviations
\def\etal{{et al. \/}}
\def\viz{{viz.,\ \/}}
\def\ie{{i.e.,\ \/}}
\def\eg{{e.g.,  }}
\def\etc{{etc.,  }}
\def\ifff{{iff  }}
\def\as{{a.s.  }}
\def\st{{s.t.  }}
\def\wpone{{w.p.}\,1\,\,}
\def\nn{\nonumber}
\def\qed{\hfill$\Box$}
\def\complx{\mathbb{C}}


%%%%%%%%%%%%%%%%%%%%%%%%%%%%%%%%%%%%%%%%%%%%%%%%%%%%%%%%%%%%%
%% LDP
%
%\def\EGnp{\tilde{E}^{\mbox{\tiny NPD}}(\lambda)}
%\def\EGB{\tilde{E}^{\mbox{\tiny BD}}(\lambda)}
%\def\EGFI{\tilde{E}^{\mbox{\tiny MLE}}(\lambda,\theta)}
%\def\trueEGnp{{E}^{\mbox{\tiny NPD}}(\lambda)}
%\def\trueEGB{{E}^{\mbox{\tiny BD}}(\lambda)}
%\def\trueEFI{{E}^{\mbox{\tiny MLE}}(\lambda,\theta)}
%\def\thetaml{\hat{\theta}_{{\mbox{\tiny MLE}}}}
%\def\nustar{\nu_{*}}
%\def\trueEB{{E}^{\mbox{\tiny D}}(\lambdabf)}
%\def\trueEF{{E}^{\mbox{\tiny E}}(\lambdabf)}
%\def\tilDlambdagamma{\tilde{D}_{\lambda,\gamma}}
%\def\tilClambdagamma{\tilde{C}_{\lambda,\gamma}}
%\def\tilD{\tilde{D}}
%\def\tilC{\tilde{C}}
%\def\delpj{\Delta p_\theta(j)}
%\def\mindet{\hat{\theta}_{\mbox{\tiny mrd}}}
%\def\minsumrate{\hat{\theta}_{\mbox{\tiny msd}}}
%\def\sprt{\mathbb{E}_{\theta_i}N_{\mbox{\tiny sprt}}(\lambda)}
%\def\smst{\mathbb{E}_{\theta_i}N_{\mbox{\tiny smst}}(\lambda)}
%\def\sprtzero{\mathbb{E}_{\theta_0}N_{\mbox{\tiny sprt}}(\lambda)}
%\def\smstzero{\mathbb{E}_{\theta_0}N_{\mbox{\tiny smst}}(\lambda)}
%\def\sprtone{\mathbb{E}_{\theta_1}N_{\mbox{\tiny sprt}}(\lambda)}
%\def\smstone{\mathbb{E}_{\theta_1}N_{\mbox{\tiny smst}}(\lambda)}
%\def\nsprt{N_{\mbox{\tiny sprt}}}
%\def\nsmst{N_{\mbox{\tiny smst}}}
%\def\diffseq{\mathbb{E}_{\theta_i}(N_{\mbox{\tiny sprt}}-N_{\mbox{\tiny
%smst}})(\lambda)}
%\def\xij{\{X_{i,j}\}}
%\def\xioneseq{\{X_{i,1}\}_{i=1}^\infty}
%\def\xinseq{\{X_{i,n}\}_{i=1}^\infty}
%\def\xij{X_{i,j}}
%\def\hione{H_{i,1}}
%\def\hitwo{H_{i,2}}
%\def\hij{H_{i,j}}
%\def\snrt{\mbox{\scriptsize{SNR}}_t}
%\def\snrr{\mbox{\small{SNR}}_r}
%\def\plim{\mbox{p}\lim}
%\def\convd{\overset{d}\rightarrow}
%\def\convp{\overset{p}\rightarrow}
%\def\convweak{\Rightarrow}
%%\def\bfptheta{\mathbf{p}_{\theta}}
%\def\pt{\mathbf{p}_{\theta}}
%\def\pti{\mathbf{p}_{\theta_i}}
%\def\ptzero{\mathbf{p}_{\theta_0}}
%\def\ptone{\mathbf{p}_{\theta_1}}
%\def\pthetai{p_{\theta_i}}
%\def\ptheta{p_{\theta}}
%\def\conv{{ \rightarrow}}
%\def\balle{\mathcal{B}_\epsilon}
%\def\thetai{\theta_i}

%%%%%%%%%%%%%%%%%%%%%%%%%%%%%%%%%%%%%%%%%%%%%%%%%%%%%%%%%%%%%



%%%%%%%%%%%%%%%%%%%%%%%%%%%%%%%%%%%%%%%%%%%%%%%%%%%%%%%%%%%%%
%presentation specs
\def\tcr{\textcolor{red}}
\def\tcb{\textcolor{blue}}
\def\tcg{\textcolor{green}}
\def\tcw{\textcolor{white}}
\def\tcm{\textcolor{magenta}}
\def\tccyan{\textcolor{cyan}}
\def\tcv{\textcolor{violet}}
\definecolor{dkr}{rgb}{0.6,0.2,0.2}
\definecolor{dkg}{rgb}{0,0.5,0}
\definecolor{dkb}{rgb}{0.0,0.1,0.7}

\def\tcdkb{\textcolor{dkb}}
\def\tcdkg{\textcolor{dkg}}
\def\tcdkr{\textcolor{dkr}}
\def\tcblack{\textcolor{black}}

%beamer
\newcommand{\ft}{\frametitle}
\newcommand{\bef}{\begin{frame}}
\newcommand{\eef}{\end{frame}}%strange doesnt work
\newcommand{\beb}{\begin{block}}
\newcommand{\eeb}{\end{block}}
\newcommand{\becs}{\begin{columns}}
\newcommand{\eecs}{\end{columns}}
\newcommand{\bec}{\begin{column}}
\newcommand{\eec}{\end{column}}

%%%%%%%%%%%%%%%%%%%%%%%%%%%%%%%%%%%%%%%%%%%%%%%%%%%%%%%%%%%%%%%%%%%%%%
%\mathscr

\newcommand{\Amsc}{\mathscr{A}}
\newcommand{\Cmsc}{\mathscr{C}}
\newcommand{\Dmsc}{\mathscr{D}}
\newcommand{\Emsc}{\mathscr{E}}
\newcommand{\Fmsc}{\mathscr{F}}
\newcommand{\Gmsc}{\mathscr{G}}
\newcommand{\Hmsc}{\mathscr{H}}
\newcommand{\Kmsc}{\mathscr{K}}
\newcommand{\Nmsc}{\mathscr{N}}
\newcommand{\Pmsc}{\mathscr{P}}
\newcommand{\Qmsc}{\mathscr{Q}}
\newcommand{\Rmsc}{\mathscr{R}}
\newcommand{\Smsc}{\mathscr{S}}
\newcommand{\Tmsc}{\mathscr{T}}
\newcommand{\Umsc}{\mathscr{U}}
\newcommand{\Xmsc}{\mathscr{X}}
\newcommand{\Ymsc}{\mathscr{Y}}

%%%%%%%%%%%%%%%%%%%%%%%%%%%%%%%%%%%%%%%%%%%%%
%bold alphabets
\def\bfzero{{\mathbf{0}}}
\def\bfone{{\mathbf{1}}}
\def\bfa{{\mathbf a}}
\def\bfb{{\mathbf b}}
\def\bfc{{\mathbf c}}
\def\bfd{{\mathbf d}}
\def\bfe{{\mathbf e}}
\def\bff{{\mathbf f}}
\def\bfg{{\mathbf g}}
\def\bfh{{\mathbf h}}
\def\bfi{{\mathbf i}}
\def\bfj{{\mathbf j}}
\def\bfk{{\mathbf k}}
\def\bfl{{\mathbf l}}
\def\bfm{{\mathbf m}}
\def\bfn{{\mathbf n}}
\def\bfo{{\mathbf o}}
\def\bfp{{\mathbf p}}
\def\bfq{{\mathbf q}}
\def\bfr{{\mathbf r}}
\def\bfs{{\mathbf s}}
\def\bft{{\mathbf t}}
\def\bfu{{\mathbf u}}
\def\bfv{{\mathbf v}}
\def\bfw{{\mathbf w}}
\def\bfx{{\mathbf x}}
\def\bfy{{\mathbf y}}
\def\bfz{{\mathbf z}}
%bold caps
\def\bfA{{\mathbf A}}
\def\bfB{{\mathbf B}}
\def\bfC{{\mathbf C}}
\def\bfD{{\mathbf D}}
\def\bfE{{\mathbf E}}
\def\bfF{{\mathbf F}}
\def\bfG{{\mathbf G}}
\def\bfH{{\mathbf H}}
\def\bfI{{\mathbf I}}
\def\bfJ{{\mathbf J}}
\def\bfK{{\mathbf K}}
\def\bfL{{\mathbf L}}
\def\bfM{{\mathbf M}}
\def\bfN{{\mathbf N}}
\def\bfO{{\mathbf O}}
\def\bfP{{\mathbf P}}
\def\bfQ{{\mathbf Q}}
\def\bfR{{\mathbf R}}
\def\bfS{{\mathbf S}}
\def\bfT{{\mathbf T}}
\def\bfU{{\mathbf U}}
\def\bfV{{\mathbf V}}
\def\bfW{{\mathbf W}}
\def\bfX{{\mathbf X}}
\def\bfY{{\mathbf Y}}
\def\bfZ{{\mathbf Z}}
%%%%%%%%%%%%%%%%%%%%%%%%%%%%%%%%%%%%%%%%%%%%%%%%%%%%%%%%%%%%%%
%bold symbols

\def\alphabf{\hbox{\boldmath$\alpha$\unboldmath}}
\def\betabf{\hbox{\boldmath$\beta$\unboldmath}}
\def\gammabf{\hbox{\boldmath$\gamma$\unboldmath}}
\def\deltabf{\hbox{\boldmath$\delta$\unboldmath}}
\def\epsilonbf{\hbox{\boldmath$\epsilon$\unboldmath}}
\def\zetabf{\hbox{\boldmath$\zeta$\unboldmath}}
\def\etabf{\hbox{\boldmath$\eta$\unboldmath}}
\def\iotabf{\hbox{\boldmath$\iota$\unboldmath}}
\def\kappabf{\hbox{\boldmath$\kappa$\unboldmath}}
\def\lambdabf{\hbox{\boldmath$\lambda$\unboldmath}}
\def\mubf{\hbox{\boldmath$\mu$\unboldmath}}
\def\nubf{\hbox{\boldmath$\nu$\unboldmath}}
\def\xibf{\hbox{\boldmath$\xi$\unboldmath}}
\def\pibf{\hbox{\boldmath$\pi$\unboldmath}}
\def\rhobf{\hbox{\boldmath$\rho$\unboldmath}}
\def\sigmabf{\hbox{\boldmath$\sigma$\unboldmath}}
\def\taubf{\hbox{\boldmath$\tau$\unboldmath}}
\def\upsilonbf{\hbox{\boldmath$\upsilon$\unboldmath}}
\def\phibf{\hbox{\boldmath$\phi$\unboldmath}}
\def\chibf{\hbox{\boldmath$\chi$\unboldmath}}
\def\psibf{\hbox{\boldmath$\psi$\unboldmath}}
\def\omegabf{\hbox{\boldmath$\omega$\unboldmath}}
\def\Sigmabf{\hbox{$\bf \Sigma$}}
\def\Upsilonbf{\hbox{$\bf \Upsilon$}}
%\def\Phibf{\hbox{$\bf \Phi$}}
%\def\Psibf{\hbox{$\bf \Psi$}}
\def\Omegabf{\hbox{$\bf \Omega$}}
\def\Deltabf{\hbox{$\bf \Delta$}}
\def\Gammabf{\hbox{$\bf \Gamma$}}
\def\Thetabf{\hbox{$\bf \Theta$}}
\def\Lambdabf{\mbox{$ \bf \Lambda $}}
\def\Xibf{\hbox{\bf$\Xi$}}
\def\Pibf{{\bf \Pi}}
%\def\thetabf{\hbox{\boldmath$\theta$\unboldmath}}
\def\thetabf{{\mbox{\boldmath$\theta$\unboldmath}}}
%\def\thetabf{\hbox{$\bf{\theta}$}}
\def\Upsilonbf{\hbox{\boldmath$\Upsilon$\unboldmath}}
\newcommand{\Phibf}{\mbox{${\bf \Phi}$}}
\newcommand{\Psibf}{\mbox{${\bf \Psi}$}}
\def\olambda{\mathfrak{o}(\lambda)}
\def\complex{\mathfrak{C}}

%%%%%%%%%%%%%%%%%%%%%%%%%%%%%%%%%%%%%%%%%%%%%%%%%%%%%%%%%%%%%%%%%%%
%Calligraphic
\def\Ac{{\cal A}}
\def\Bc{{\cal B}}
\def\Cc{{\cal C}}
\def\Dc{{\cal D}}
\def\Ec{{\cal E}}
\def\Fc{{\cal F}}
\def\Gc{{\cal G}}
\def\Hc{{\cal H}}
\def\Ic{{\cal I}}
\def\Jc{{\cal J}}
\def\Kc{{\cal K}}
\def\Lc{{\cal L}}
\def\Mc{{\cal M}}
\def\Nc{{\cal N}}
\def\Oc{{\cal O}}
\def\Pc{{\cal P}}
\def\Qc{{\cal Q}}
\def\Rc{{\cal R}}
\def\Sc{{\cal S}}
\def\Tc{{\cal T}}
\def\Uc{{\cal U}}
\def\Vc{{\cal V}}
\def\Wc{{\cal W}}
\def\Xc{{\cal X}}
\def\Yc{{\cal Y}}
\def\Zc{{\cal Z}}

%%%%%%%%%%%%%%%%%%%%%%%%%%%%%%%%%%%%%%%%%%%%%%%%%%%%%%%%%%%%%%%%%%%
%mathbb
\def\Abb{{\mathbb A}}
\def\BBb{{\mathbb B}}% different
\def\Cbb{{\mathbb C}}
\def\Dbb{{\mathbb D}}
\def\Ebb{{\mathbb E}}
\def\Fbb{{\mathbb F}}
\def\Gbb{{\mathbb G}}
\def\Hbb{{\mathbb H}}
\def\Ibb{{\mathbb I}}
\def\Jbb{{\mathbb J}}
\def\Kbb{{\mathbb K}}
\def\Lbb{{\mathbb L}}
\def\Mbb{{\mathbb M}}
\def\Nbb{{\mathbb N}}
\def\Obb{{\mathbb O}}
\def\Pbb{{\mathbb P}}
\def\Qbb{{\mathbb Q}}
\def\Rbb{{\mathbb R}}
\def\Sbb{{\mathbb S}}
\def\Tbb{{\mathbb T}}
\def\Ubb{{\mathbb U}}
\def\Vbb{{\mathbb V}}
\def\Wbb{{\mathbb W}}
\def\Xbb{{\mathbb X}}
\def\Ybb{{\mathbb Y}}
\def\Zbb{{\mathbb Z}}

%%%%%%%%%%%%%%%%%%%%%%%%%%%%%%%%%%%%%%%%%%%%
%command abbreviations
\newcommand{\bp}{\begin{psfrags}}
\newcommand{\ep}{\end{psfrags}}
\newcommand{\bl}{\begin{lemma}}
\newcommand{\el}{\end{lemma}}
\newcommand{\bt}{\begin{theorem}}
\newcommand{\et}{\end{theorem}}
\newcommand{\bc}{\begin{center}}
\newcommand{\ec}{\end{center}}
\newcommand{\bi}{\begin{itemize}}
\newcommand{\ei}{\end{itemize}}
\newcommand{\ben}{\begin{enumerate}}
\newcommand{\een}{\end{enumerate}}
%\newcommand{\bd}{\begin{definition}}
\newcommand{\ed}{\end{definition}}
\def\beq{\vskip .1cm \begin{equation}}
\def\eeq{\end{equation} \vskip .1cm \noindent}
\def\beqn{\vskip .1cm \begin{eqnarray}}
\def\eeqn{\end{eqnarray} \vskip .1cm \noindent}
\def\beqnn{\vskip .01cm \begin{eqnarray*}}
\def\eeqnn{\end{eqnarray*} \vskip .01cm \noindent}
\def\endproof{\hfill\blacksquare}
\def\defeq{:=}
\newcommand{\bim}{\begin{mylist}}
\newcommand{\eim}{\end{mylist}}
\def\bcase{\vskip .1cm \begin{numcases}}
\def\ecase{\end{numcases} \vskip .1cm \noindent}
\def\bsbcase{\vskip .1cm \begin{subnumcases}}
\def\esbcase{\end{subnumcases} \vskip .1cm \noindent}
%%%%%%%%%%%%%%%%%%%%%%%%%%%%%%%%%%%%%%%%%%%%%%%%%%%%%%%%%%%%%%
%theorems

%\newtheorem{theorem}{Theorem}
%\newtheorem{corollary}{Corollary}
%\newtheorem{lemma}{Lemma}
%\newtheorem{definition}{Definition}
%\newtheorem{problem}{Problem}
%\newtheorem{assumption}{A}
%\newtheorem{properties}{Properties}
%\newtheorem{conjecture}{Conjecture}
%\newtheorem{criterion}{Criterion}
%\newtheorem{proposition}{Proposition}
%\newtheorem{remark}{Remark}
%\newtheorem{notation}{Notation}
%\newtheorem{derivation}{Derivation}
%\newtheorem{proof}{Proof}
\newtheorem{claim}{Claim}

%%%%%%%%%%%%%%%%%%%%%%%%%%%%%%%%%%%%%%%%%%%%%%%%%%%%%%%%%%%%%%%%%%%%%%%%%%%%%%%%%

\newcommand{\matplottc}[1]{               % single matlab plot twocolumn
        \unitlength .45truein
        \begin{center}
        \begin{picture}(5,4.6)(1.05,.45)
        \special{psfile=#1.ps hscale=50 vscale=50}
        \end{picture}
        \end{center}
}
\newcommand{\matplotfp}[1]{               % single matlab plot fullpage
        \unitlength .45truein
        \begin{center}
        \begin{picture}(14,16)(.8,-1)
        \special{psfile=#1.ps hscale=100 vscale=100}
        \end{picture}
        \end{center}
}
\newcommand{\matplothp}[1]{               % single matlab plot halfpage
        \unitlength .45truein
        \begin{center}  \begin{picture}(14,7.5)(-1,.55)
        \special{psfile=#1.ps hscale=80 vscale=80}
        \end{picture}
        \end{center}
}
\newcommand{\matplothptop}[1]{               % single matlab plot halfpage
        \unitlength .45truein                % when figure is top of page
        \begin{center}  \begin{picture}(14,6.3)(-1,1.15)
        \special{psfile=#1.ps hscale=80 vscale=80}
        \end{picture}
        \end{center}
}
\newcommand{\matplotcc}[4]{             % two axis('square') plots side by side
        \vspace{2.8in}
        \special{psfile=#1.ps voffset=-10 hoffset=-22 vscale=52 hscale=52}
        \special{psfile=/user/xu/isl/matlab/psfiles/#2.ps voffset=-10 hoffset=213 vscale=52 hscale=52}
        \hspace*{\fill}\hspace*{0.35in}#3\hspace*{\fill}\hspace*{\fill}\hspace*{
0.35in}#4\hspace*{\fill} }
\newcommand{\matplottwo}[4]{             % two axis('normal') plots side by side
        \vspace{2.62in}
        \special{psfile=#1.ps voffset=-10 hoffset=-27 vscale=52 hscale=52}
        \special{psfile=#2.ps voffset=-10 hoffset=218 vscale=52 hscale=52}
        \vspace*{0.18in}
        \hspace*{\fill}\hspace*{-.05in}#3\hspace*{\fill}\hspace*{\fill}\hspace*{
0.65in}#4\hspace*{\fill} } %%
%% This is for making fancy paragraphs
%%
\def\psfancypar#1#2{\begingroup\def\par{\endgraf\endgroup\lineskiplimit=0pt}
               \setbox2=\hbox{\large\sc #2}
%              \showthe\lht2\showthe\baselineskip
               \newdimen\tmpht \tmpht \ht2 \advance\tmpht by \baselineskip
%              \showthe\tmpht
% Changed 10/2/89 rhr - t-bol -> Times-Bold for dvi2ps to dvips conversion
%              \font\hhuge=t-bol at \tmpht
               \font\hhuge=Times-Bold at \tmpht
               \setbox1=\hbox{{\hhuge #1}}
%              \showthe\ht1
               \count7=\tmpht \count8=\ht1
%  note that all this BS is necessary since TeX only does integer
%  divides and rounds all results
               \divide\count8 by 1000 \divide\count7 by \count8
%               \showthe\count7
               \tmpht=.001\tmpht\multiply\tmpht by \count7
%               \showthe\tmpht
%              \font\hhuge=t-bol at \tmpht
               \font\hhuge=Times-Bold at \tmpht
               \setbox1=\hbox{{\hhuge #1}}
               \noindent
                \hangindent1.05\wd1
               \hangafter=-2 {\hskip-\hangindent
               \lower1\ht1\hbox{\raise1.0\ht2\copy1}%
                \kern-0\wd1}\copy2\lineskiplimit=-1000pt}


\newenvironment{ap}{
\renewcommand{\thesection}{\mbox{Appendix }\Alph{section}}
\renewcommand{\thesubsection}{\Alph{section}.\arabic{subsection
}}
\renewcommand{\theequation}{\mbox{\Alph{section}.}\arabic{equation}}
}{
\renewcommand{\thesection}{\arabic{section}}
\renewcommand{\thesubsection}{\thesection.\arabic{subsection}}
\renewcommand{\theequation}{\arabic{equation}}
}
%\setlength{\footnoterulewidth}{0.5pt}

%\setlength{\floatsep}{0.1cm}

%\setlength{\textfloatsep}{0.1cm}

%\setlength{\intextsep}{0.1cm}

%\setlength{\abovecaptionskip}{0.1cm}
%
%\setlength{\belowcaptionskip}{0.1cm}
%
%\setlength{\topsep}{0.1cm}
%
%\setlength{\partopsep}{0.1cm}
%
%\setlength{\itemsep}{0.1cm}
%
\setlength{\parindent}{0mm}
%
%\setlength{\dbltextfloatsep}{0.1cm}
%
%\setlength{\dblfloatsep}{0.1cm}
%
%\addtolength{\abovedisplayskip}{-1.5em}
%
%\addtolength{\belowdisplayskip}{-1.5em}
%
%\setlength{\arraycolsep}{0.1cm}

%\def\boxit#1{\vbox{\hrule\hbox{\vrule\kern3pt
%        \vbox{\kern3pt#1\kern3pt}\kern3pt\vrule}\hrule}}
%\def\dag{{\cal y}}
%\def\reals{ { {\rm  I \kern-0.15em R }  } }
%\def\complex{ {\,{{\rm C} \kern-0.50em \raise0.20ex {  |}}\, }}


%
%\newtheorem{theorem}{Theorem}[chapter]
%\newtheorem{conjecture}{Conjecture}[chapter]
%\newtheorem{lemma}{Lemma}[chapter]
%\newtheorem{definition}{Definition}[chapter]
%\newtheorem{corollary}{Corollary}[chapter]


%\newcounter{remarknr}[chapter]
%\newenvironment{remark}{\vskip\baselineskip
%\stepcounter{remarknr}\noindent{\bf
%Remark~\theremarknr.}}{\ \hfill $\Box$ \vskip\baselineskip}
%\newcounter{examplenr}[chapter]
%\newenvironment{example}[1]{\vskip\baselineskip
%\stepcounter{examplenr}\noindent{{\bf
%Example~\thechapter.\theexamplenr}\hskip .8em #1\\}}{\ \hfill $\Box$
%\vskip\baselineskip}




%\newcommand{\x}{\mbox{${\bf x}(t)$}}
%\newcommand{\s}{\mbox{${\bf s}(t)$}}
%\newcommand{\n}{\mbox{${\bf n}(t)$}}
%\newcommand{\jj}{\mbox{${\bf j}(t)$}}
%\newcommand{\R}{\mbox{$\hat {\bf R}_{N}$}}
%\newcommand{\Rhat}{\mbox{$\hat {\bf R}$}}
%\newcommand{\A}{\mbox{${\cal A}$}}
%\newcommand{\Ad}{\mbox{${\cal A}^d$}}
%\newcommand{\D}{\mbox{${\cal D}$}}
%\newcommand{\M}{\mbox{{\bf M}}}
%\newcommand{\Tr}{\mbox{Tr}}
%\newcommand{\pbox}{\hfill $\Box$}
%\newcommand{\blankline}{\vskip\baselineskip\noindent}
%\def\Rxx{\Rbf_{\ssstyle X\kern-.1em X}}
%\def\rxx{\hbox{$\Rxx$}}
%\def\ryy{\hbox{$\Rbf_{\ssstyle YY}$}}
%\def\rxy{\hbox{$\Rbf_{\ssstyle XY}$}}\def\ryx{\hbox{$\Rbf_{\ssstyle YX}$}}
%\def\rxyT{\hbox{$\Rbf_{\ssstyle XY}^*$}}\def\ryxT{\hbox{$\Rbf_{\ssstyle YX}^*$}}
%\def\Rss{\Rbf_{\ssstyle SS}}
%\def\rss{\mbox{$\Rss$}}
%\def\Rnn{\Rbf_{\ssstyle NN}}
%\def\rnn{\hbox{$\Rnn$}}
%\def\rxxinv{\hbox{$\Rbf^{-1}_{\ssstyle XX}$}}
%\def\Rssinv{\Rbf^{-1}_{\ssstyle SS}}
%\def\rssinv{\hbox{$\Rssinv$}}
%\def\rzzinv{\Rbf^{-1}_{\ssstyle ZZ}}\let\rzzi=\rzzinv
%\def\hatrxx{\widehat{\Rbf}_{\ssstyle XX}}
%\def\hatrzz{\widehat{\Rbf}_{\ssstyle ZZ}}
%\def\hatrss{\widehat{\Rbf}_{\ssstyle SS}}
%\def\phstar{{\phantom{*}}}
%\let\rzzhat=\hatrzz \let\rxxhat=\hatrxx \let\Rxxhat=\rxxhat
%\let\ssstyle=\scriptscriptstyle
%\let\rsshat=\hatrss


% I add the following!
%\def\eqorneq{=\!\!\!\! ? \,\,}
%\def\ltornlt{? \!\!\!\!\! <}
%\def\sN{{\ssstyle N}}
%\def\sM{{\ssstyle M}}
%\def\sF{{\ssstyle F}}
%\def\sT{{\ssstyle T}}
%\def\sH{{\ssstyle H}}
%\def\sK{{\ssstyle K}}
%\def\sL{{\ssstyle L}}
%\def\sQ{{\ssstyle Q}}
%\def\sV{{\ssstyle V}}
%\def\cross{\!  \times  \!}
%\def\alphat{\alpha^{(t)}}
%\def\alphab{\alpha^{(b)}}
%\def\betat{\beta^{(t)}}
%\def\betab{\beta^{(b)}}
%\def\ATbf{{\bf A_\sT}}
%\def\AHbf{{\bf A_\sH}}
%\def\sspan{\mbox{\it span}}



\def\Kout{\setbox1=\hbox{\Huge\bf K}\hbox to
1.05\wd1{\hspace{.05\wd1}\special{
"/Times-BoldItalic findfont 25 scalefont setfont
/prKzip
{0 0 moveto (K) show} def
/dozip
{gsave
  /xp 0 def
  .08 -.04 0
  {
   setgray
  prKzip
%  /xp xp dx add def xp -.7 translate %for
  -.7 .4 translate} for
  1 setgray prKzip
  0 0 moveto
  0 setgray
  .5 setlinewidth
  (K) true charpath  stroke
 grestore
} def
dozip}}}
\def\Sout{\setbox1=\hbox{\Huge\bf S}\hbox to 1.05\wd1{\hspace{.05\wd1}\special{"
/Times-BoldItalic findfont 25 scalefont setfont
/prSzip
{0 0 moveto (S) show} def
/dozip
{gsave
  /xp 0 def
  .08 -.04 0
  {
   setgray
  prSzip
%  /xp xp dx add def xp -.7 translate %for
  -.7 .4 translate} for
  1 setgray prSzip
  0 0 moveto
  0 setgray
  .5 setlinewidth
  (S) true charpath  stroke
 grestore
} def
dozip}}}

%\newcommand{\thhat}{\mbox{${\hat{\thetabf}}_N$}}
%\newcommand{\thbar}{\mbox{${\bar{\thetabf}}_N$}}
%\newcommand{\etahat}{\mbox{${\hat{\etabf}}$}}
%\newcommand{\etabf}{\mbox{${\bf\eta}$}}
%\newcommand{\e}{\mbox{${\bf e}_k$}}
%\newcommand{\ehat}{\mbox{$\hat{\bf e}_k$}}
%\newcommand{\EWE}{\mbox{${\bf E}_s^{}{\bf WE}_s^*$}}
%\newcommand{\DPD}{\mbox{$\Dbf^*\Pbf_{\bf A}^{\perp} \Dbf$}}
%\newcommand{\EWEhat}{\mbox{$\hat{\bf E}_s^{}{\bf W}\hat{\bf E}_s^*$}}
%\newcommand{\E}{\mbox{{\rm E}}}
%\newcommand{\Efs}{\mbox{${\bf E}_s^{}$}}
%\newcommand{\En}{\mbox{${\bf E}_n^{}$}}
%\newcommand{\Eshat}{\mbox{$\hat{\bf E}_s^{}$}}
%\newcommand{\Lshat}{\mbox{$\hat {\bf \Lambda}_s^{}$}}
%\newcommand{\Ls}{\mbox{$ {\bf \Lambda}_s^{}$}}
%\newcommand{\Ln}{\mbox{$ {\bf \Lambda}_n^{}$}}
%\newcommand{\Ltilde}{\mbox{$\widetilde {\bf \Lambda}$}}
%\newcommand{\Enhat}{\mbox{$\hat{\bf E}_n^{}$}}
%\newcommand{\Lnhat}{\mbox{$\hat {\bf \Lambda}_n^{}$}}
%\newcommand{\Ai}{\mbox{$ ({\bf A}^*{\bf A})^{-1} $}}
%\newcommand{\abf}{\mbox{${\bf a}$}}


%Define affiliation at footnote
% Make \small be smaller (8 pt)
%\def\small{\@setsize\small{9pt}\viiipt\@viiipt\let\@listi\@listI}


%%%%% notation %%%%%
%Anima added
\DeclareMathOperator{\Map}{Map}
\def\convp{{\stackrel{\mathrm{P}}{\to}}}

\def\qed{\hfill\hbox{${\vcenter{\vbox{
    \hrule height 0.4pt\hbox{\vrule width 0.4pt height 6pt
    \kern5pt\vrule width 0.4pt}\hrule height 0.4pt}}}$}}

\def\Depth{\delta}
\def\Hops{{\mbox{Hops}}}

% Variables
\newcommand{\wloc}{W} % graph
\newcommand{\loc}{L}
\newcommand{\wpre}{c}
%\newcommand{\neighbors}{\mathcal{N}}
%\newcommand{\clneighbors}{\mathcal{N}^{CL}}
%\newcommand{\nodes}{\mathcal{V} \cup \mathcal{H}}
%\newcommand{\onodes}{\mathcal{V}}
%\newcommand{\hnodes}{\mathcal{H}}
%\newcommand{\inodes}{\mathcal{I}}

\newcommand{\rc}{r}
\newcommand{\idtree}{\mathcal{T}_I}
\newcommand{\tree}{T}
\newcommand{\cltree}{\tree^{CL}}
\newcommand{\subtree}{\mathcal{S}}

% Vincent added
\newcommand{\calV}{\mathcal{V}}
\newcommand{\WW}{W}
\newcommand{\calE}{\mathcal{E}}
\newcommand{\calX}{\mathcal{X}}
\newcommand{\calA}{\mathcal{A}}
\newcommand{\calB}{\mathcal{B}}
\newcommand{\bX}{\mathbf{X}}
\newcommand{\bK}{\mathbf{K}}
\newcommand{\bx}{\mathbf{x}}
\newcommand{\bd}{\mathbf{d}}
\newcommand{\calH}{\mathcal{H}}
\newcommand{\hp}{\hat{p}}
\newcommand{\hd}{\hat{d}}
\newcommand{\hPhi}{\hat{\Phi}}
\newcommand{\hbd}{\hat{\bd}}
\newcommand{\hmu}{\hat{\mu}}
\newcommand{\calG}{\mathcal{G}}
\newcommand{\calC}{\mathcal{C}}
\newcommand{\calD}{\mathcal{D}}
\newcommand{\calT}{\mathcal{T}}
\newcommand{\bN}{\mathbb{N}}
\newcommand{\hT}{\hat{T}}
\newcommand{\ML}{\mathrm{ML}}
\newcommand{\Sg}{\mathrm{Sg}}
\newcommand{\calO}{\mathcal{O}}
%\newcommand{\Path}{\mathrm{Path}}
\newcommand{\diam}{\mathrm{diam}}
\newcommand{\MST}{\mathrm{MST}}
\newcommand{\Leaf}{\mathrm{Leaf}}
\newcommand{\brho}{\bm{\rho}}
\newcommand{\bSigma}{\bm{\Sigma}}
\newcommand{\bDelta}{\bm{\Delta}}
%\newcommand{\nbd}{\mathrm{nbd}}
\newcommand{\bR}{\mathbb{R}}

%\DeclareMathOperator*{\argmax}{argmax}
%\DeclareMathOperator*{\argmin}{argmin}

\newtheorem{THEO}{\bf Theorem}
\newtheorem{CORL}[THEO]{\bf Corollary}
\newtheorem{LEMM}[THEO]{\bf Lemma}
\newtheorem{REMA}{\bf Remark}
\newtheorem{DEFI}{\bf Definition}
\newtheorem{CLAIM}{\bf Claim}
\newtheorem{PROP}[THEO]{\bf Proposition}
\newtheorem{PROOF}{\bf Proof}
\newtheorem{EXAMPLE}{\bf Example}
\newtheorem{FACT}{\bf Fact}


\newcommand{\mathdef}{:=}
\DeclareMathOperator{\Tr}{Tr}
\DeclareMathOperator{\mat}{mat}
\DeclareMathOperator{\Rank}{Rank}

\def\nbd{\mathcal{N}}
\def\Path{{\mathrm{Path}}}

\DeclareMathOperator{\dist}{dist}
\DeclareMathOperator{\polylog}{polylog}
\def\veps{\varepsilon}
%\newcommand{\calX}{\mathcal{X}}
%\newcommand{\qed}{\hfill \ensuremath{\Box}}
%\newcommand{\bX}{\mathbf{X}}
\newcommand{\by}{\mathbf{y}}
\newcommand{\ba}{\mathbf{a}}
%\newcommand{\calG}{\mathcal{G}}
\newcommand{\calS}{\mathcal{S}}
\newcommand{\calN}{\mathcal{N}}
%\renewcommand{\calE}{E}
\newcommand{\hcalU}{\widehat{\mathcal{U}}}
%\renewcommand{\calV}{V}
%\newcommand{\calB}{\mathcal{B}}
%\newcommand{\calT}{\mathcal{T}}
%\newcommand{\calA}{\mathcal{A}}
%\newcommand{\calD}{\mathcal{D}}
%\newcommand{\bx}{\mathbf{x}}
%\newcommand{\0}{\mathbf{0}}
%\newcommand{\bR}{\mathbb{R}}
\newcommand{\calP}{\mathcal{P}}
\newcommand{\calY}{\mathcal{Y}}
%\newcommand{\calH}{\mathcal{H}}
\newcommand{\calU}{\mathcal{U}}
\newcommand{\bP}{\mathbb{P}}
\newcommand{\bE}{\mathbb{E}}
\newcommand{\bL}{\mathbf{L}}
%\newcommand{\bSigma}{\bm{\Sigma}}
\newcommand{\bmeta}{\bm{\eta}}
\newcommand{\bs}{\mathbf{s}}
\newcommand{\bxi}{\bm{\xi}}
%\newcommand{\bK}{\mathbf{K}}
\newcommand{\bzero}{\mathbf{0}}
\newcommand{\one}{\mathbf{1}}
%\newcommand{\hp}{\widehat{p}}
%\newcommand{\argmin}{\operatornamewithlimits{argmin}}
%\newcommand{\argmax}{\operatornamewithlimits{argmax}}
\newcommand{\hP}{\widehat{P}}
\newcommand{\hrho}{\widehat{\rho}}
\newcommand{\hPML}{{P}_{{\text{\tiny ML}}}}
\newcommand{\hI}{\widehat{I}}
\newcommand{\hQ}{\widehat{Q}}
\newcommand{\PML}{P_{\mathrm{ML}}}
\newcommand{\hTML}{{T}_{\text{\tiny ML}}}
%\newcommand{\Path}{\mathrm{Path}}
\newcommand{\tilp}{\widetilde{p}}
\newcommand{\tilJ}{\widetilde{J}}
\newcommand{\tilP}{\widetilde{P}}
\newcommand{\tilQ}{\widetilde{Q}}
\newcommand{\tilK}{\widetilde{K}}
\newcommand{\beps}{\bm{\epsilon}}
\newcommand{\var}{\mathrm{Var}}
%\newcommand{\etal}{et al.\ }
\newcommand{\hcalE}{{\calE}_{{\text{\tiny ML}}}}

\newcommand{\boxedeqn}[1]{%
  \[\fbox{%
      \addtolength{\linewidth}{-2\fboxsep}%
      \addtolength{\linewidth}{-2\fboxrule}%
      \begin{minipage}{\linewidth}%
      \begin{equation}#1\end{equation}%
      \end{minipage}%
    }\]%
}

\newtheorem*{theo}{Theorem}
\newtheorem*{proposition}{Proposition} 

\renewcommand{\thefootnote}{}





\newcommand{\fhcomment}{\textcolor[rgb]{1,0,0}{FH: }\textcolor[rgb]{1,0,0}} 
\renewcommand{\thefootnote}{}
\DeclareMathOperator{\Pairs}{Pairs}
\newcommand{\llvert}{\left\vert\vphantom{\frac{1}{1}}\right.}
\newcommand{\Pvalue}{\mathsf{P_{\text{val}}}}
\newcommand{\HRule}{\rule{\linewidth}{0.1mm}}
\def\nbd{\mathcal{N}}
\def\Path{{\mathrm{Path}}}

\def\veps{\varepsilon}
\newcommand{\Toep}{\mathsf{Cir}}
\DeclareMathOperator{\opt}{opt}
\newcommand{\DFT}{\mathsf{FFT}}
\newcommand*{\hermconj}{^{\mathsf{H}}}
\newcommand\supp{\operatorname{supp}}
\renewcommand{\thefootnote}{}
\def\veps{\varepsilon}
\DeclareMathOperator{\Cum}{C_3}
\DeclareMathOperator{\myblock}{blk}
\def\nbd{\mathcal{N}}
\def\Path{{\mathrm{Path}}}
\newcommand{\thetastar}{\ensuremath{\theta^*}}
\newcommand{\Astar}{\ensuremath{A^*}}
\newcommand{\Xstar}{\ensuremath{X^*}}
\newcommand{\iprod}[2]{\langle #1, #2 \rangle}
\newcommand{\Aiter}[1][t]{\ensuremath{A(#1)}}
\newcommand{\Aiteri}[1][t]{\ensuremath{A_i(#1)}}
\newcommand{\R}{\ensuremath{\mathbb{R}}}
\newcommand{\order}{\ensuremath{\mathcal{O}}}
\newcommand{\Xiter}[1][t]{\ensuremath{X(#1)}}
\newtheorem{assumption}{Assumption}
\newtheorem{goal}{Goal}
\newcommand{\Nb}{\text{nbd}}
\DeclareMathOperator{\Adj}{\mathcal{N}}
\def\ourframework{{$\textsf{ConvDic}$$+$$\textsf{DeconvDec}$ }}



% Definitions in paper
\newcommand*{\mytensor}[1]{\bm{\mathcal{#1}}}
\newcommand*{\mymatrix}[1]{\bm{#1}}
\newcommand*{\myvector}[1]{\bm{#1}}
\newcommand*{\noise}[1]{\widehat{#1}}
\newcommand*{\mm}{\mymatrix}
\newcommand*{\mv}{\myvector}
\newcommand{\mt}{\mytensor}
\newcommand*{\mmCols}[2]{\mm{#1}_{[#2]}}
% names
\newcommand{\ourmod}{{GIM}\xspace}
\newcommand{\ourmodfull}{{Greedy Inference Model}\xspace}
\newcommand{\dmname}{{dynamic matrix}\xspace}
\newcommand{\dmnames}{{dynamic matrices}\xspace}
\newcommand{\avgrew}{{AvgReward}\xspace}
\newcommand{\pavgrew}{{PostAvgReward}\xspace}
\newcommand{\numepi}{{TotalEps}\xspace}
\newcommand{\walkname}{{$\beta$-curious walking}\xspace}

% about dynamic matrices
\newcommand{\states}{\mathcal{S}}
\newcommand{\actions}{\mathcal{A}}
\newcommand{\dmat}{\mymatrix{M}}
\newcommand{\dmats}{M}
\newcommand{\admat}{\mymatrix{\hat{M}}}
\newcommand{\rdmat}{\mymatrix{\widetilde{M}}}
\newcommand{\rdmats}{\widetilde{M}}
\newcommand{\dmatset}{\{\mymatrix{M}^k\}_{k=1}^{S+1}}
\newcommand{\admatset}{\{\mymatrix{\hat{M}}^k\}_{k=1}^{S+1}}
\newcommand{\rdmatset}{\{\mymatrix{\widetilde{M}}^k\}_{k=1}^{S+1}}
\newcommand{\krange}{1,2,\cdots,S+1}


% about mask
\newcommand{\mask}{\mymatrix{P}^\mathcal{K}}
\newcommand{\masks}{P^\mathcal{K}}
\newcommand{\kset}{\mathcal{K}}
\newcommand{\nkset}{\bar{\mathcal{K}}}

% about noise
\newcommand{\noiset}{\mytensor{Z}}
\newcommand{\noisem}{\mymatrix{Z}}
\newcommand{\noises}{Z}

\newcommand{\fraction}{\rho}

\newcommand{\minsa}{M_{in}}
\newcommand{\maxsa}{M_{ax}}

\DeclareMathOperator*{\minimize}{\text{minimize}}

\DeclareMathOperator*{\argmax}{arg\,max}
\DeclareMathOperator*{\argmin}{arg\,min}
