# Supplementary material for: Can Agents Learn by Analogy? An Inferable Model for PAC Reinforcement Learning
Source: arXiv:1912.10329 source file (2020-02-24)
Supplement: Supplementary file 6 [file supp_packages.tex]

\usepackage[mathscr]{eucal}
\usepackage{bm,verbatim,pifont,color,amssymb,amsfonts,amsmath,graphicx,epsf,psfrag,ifpdf,xmpmulti,cases,hyperref}
% \usepackage{slashbox}
\usepackage[english]{babel}
\usepackage[fleqn,tbtags]{mathtools}
\usepackage{amsmath}
\usepackage[attachfiles]{media9}
\usepackage{mathtools}
\usepackage{media9}
%\usepackage{multimedia}
\usepackage{pgfpages}
\usepackage{siunitx}
\usepackage{tablefootnote}
\usepackage{xspace}

\usepackage{tikz}
\usetikzlibrary{fit}
\usetikzlibrary{calc,shapes}
\usetikzlibrary{decorations.pathmorphing} % noisy shapes
\usetikzlibrary{fit}					% fitting shapes to coordinates
\usetikzlibrary{backgrounds}	% drawing the background after the foreground
%pgfplots
\usepackage[utf8]{inputenc}
% \usepackage{fontspec}  % optional
\usepackage{pgfplots}
\pgfplotsset{compat=newest}
\usepgfplotslibrary{groupplots}
\usepgfplotslibrary{dateplot}

\usepackage{tcolorbox}
\usepackage{pgfpages}
%\usecolortheme{seagull}
%\definecolor{uofsgreen}{rgb}{.125,.5,.25}
%\usecolortheme[named=orange]{structure}
%\usecolortheme{rose}
%\usecolortheme{lily}
%\usecolortheme{rose}
%\usecolortheme{dolphin}
%\usecolortheme[rgb={0,0.17,0.45}]{structure}


%\usecolortheme{default}
%\usepackage[english]{babel}
% or whatever

%\usepackage[latin1]{inputenc}
% or whatever

\usepackage{colortbl}
%\usepackage{times}
%\usepackage[T1]{fontenc}
\usepackage{multimedia}
%\usepackage{latexsym, amssymb, amsmath}
%\setcounter{tocdepth}{3}
%\usepackage{graphicx}
%\usepackage{url}
%\usepackage{color}
%\usepackage{bm}
\usepackage{multirow}

%\usecolortheme{whale}
% \usecolortheme{beetle}
%\usecolortheme[named=seahorse]{structure}
%seahorse% seagull %beaver  albatross % lily %albatross %beetle %whale %crane
%\usecolortheme{default}
%\usepackage[english]{babel}
% or whatever
%
%\usepackage[latin1]{inputenc}
% or whatever
%
%\usepackage[lined, algonl, boxed]{algorithm2e}

\usepackage{algorithmic}
\usepackage{algorithm}
%\usepackage{subfigure}
%\usepackage{times}
%\usepackage[T1]{fontenc}
%\usepackage{hyperref}
%\usepackage{multimedia}
%\usepackage{latexsym, amssymb, amsmath}
%\setcounter{tocdepth}{3}
%\usepackage{graphicx}
%\usepackage{url}
%\usepackage{color}
%\usepackage{bm}
